# Supplementary material for: On the Predictive Accuracy of Neural Temporal Point Process Models for Continuous-time Event Data
Source: arXiv:2306.17066 source file (2023-07-10)
Supplement: Supplementary file 1 [file cd_diagrams_appendix.tex]

\begin{center} 
\begin{figure}[h!]
\centering
     \begin{subfigure}[b]{0.49\textwidth}
         \centering
         \includegraphics[width=\textwidth]{images/cd_diag/stat_tests_holm_TimeCal._marked_TOLTOCONCATLCONCATTEMTEMWLLELEWL.json.png}
     \end{subfigure}
     \hfill
     \begin{subfigure}[b]{0.49\textwidth}
         \centering
         \includegraphics[width=\textwidth]{images/cd_diag/stat_tests_holm_TimeCal._unmarked_TOLTOTEMLE.json.png}
     \end{subfigure}
    \vfill
    \vspace{-1.2cm}
    \begin{subfigure}[b]{0.49\textwidth}
         \centering
         \includegraphics[width=\textwidth]{images/cd_diag/stat_tests_holm_TimeCal._marked_GRUSAC-.json.png}
     \end{subfigure}
     \hfill
     \begin{subfigure}[b]{0.49\textwidth}
         \centering
         \includegraphics[width=\textwidth]{images/cd_diag/stat_tests_holm_TimeCal._unmarked_GRUSAC-.json.png}
     \end{subfigure}
     \vfill
     \vspace{-1.2cm}
    \begin{subfigure}[b]{0.49\textwidth}
         \centering
         \includegraphics[width=\textwidth]{images/cd_diag/stat_tests_holm_TimeCal._marked_CPLNMMLPCMMLPMCRMTPPSACMSAMCHawkesPoisson.json.png}
     \end{subfigure}
     \hfill
     \begin{subfigure}[b]{0.49\textwidth}
         \centering
         \includegraphics[width=\textwidth]{images/cd_diag/stat_tests_holm_TimeCal._unmarked_CPLNMMLPCMMLPMCRMTPPSACMSAMCHawkesPoisson.json.png}
     \end{subfigure}
     \vfill\vspace{-1.2cm}
     \begin{subfigure}[b]{0.49\textwidth}
         \centering
         \includegraphics[width=\textwidth]{images/cd_diag/stat_tests_holm_TimeCal._marked_+ BNo B.json.png}
     \end{subfigure}
     \hfill
     \begin{subfigure}[b]{0.49\textwidth}
         \centering
         \includegraphics[width=\textwidth]{images/cd_diag/stat_tests_holm_TimeCal._unmarked_+ BNo B.json.png}
     \end{subfigure}
     \vfill\vspace{-1.2cm}
\label{fig:class_reddit_lasftm}
\caption{Critical Distance (CD) diagrams per component on the TCE for marked (left-hand column) and unmarked (right-hand column) datasets. A bold line joins models variations that are not statistically different.}
\label{Distribution}
\end{figure}
\end{center}

\vspace{-1cm}
\begin{center} 
\begin{figure}[h!]
\centering
     \begin{subfigure}[b]{0.32\textwidth}
         \centering
         \includegraphics[width=\textwidth]{images/cd_diag/stat_tests_holm_NLLMark_marked_TOLTOCONCATLCONCATTEMTEMWLLELEWL.json.png}
     \end{subfigure}
     \hfill
     \begin{subfigure}[b]{0.32\textwidth}
         \centering
         \includegraphics[width=\textwidth]{images/cd_diag/stat_tests_holm_MarkCal._marked_TOLTOCONCATLCONCATTEMTEMWLLELEWL.json.png}
     \end{subfigure}
    \hfill
    \begin{subfigure}[b]{0.32\textwidth}
         \centering
         \includegraphics[width=\textwidth]{images/cd_diag/stat_tests_holm_F1-score_marked_TOLTOCONCATLCONCATTEMTEMWLLELEWL.json.png}
     \end{subfigure}
     \vfill\vspace{-0.8cm}
     \begin{subfigure}[b]{0.32\textwidth}
         \centering
         \includegraphics[width=\textwidth]{images/cd_diag/stat_tests_holm_NLLMark_marked_GRUSAC-.json.png}
     \end{subfigure}
     \hfill
     \begin{subfigure}[b]{0.32\textwidth}
         \centering
         \includegraphics[width=\textwidth]{images/cd_diag/stat_tests_holm_MarkCal._marked_GRUSAC-.json.png}
     \end{subfigure}
    \hfill
    \begin{subfigure}[b]{0.32\textwidth}
         \centering
         \includegraphics[width=\textwidth]{images/cd_diag/stat_tests_holm_F1-score_marked_GRUSAC-.json.png}
     \end{subfigure}
    \vfill\vspace{-0.8cm}
     \begin{subfigure}[b]{0.32\textwidth}
         \centering
         \includegraphics[width=\textwidth]{images/cd_diag/stat_tests_holm_NLLMark_marked_CPLNMMLPCMMLPMCRMTPPSACMSAMCHawkesPoisson.json.png}
     \end{subfigure}
     \hfill
     \begin{subfigure}[b]{0.32\textwidth}
         \centering
         \includegraphics[width=\textwidth]{images/cd_diag/stat_tests_holm_MarkCal._marked_CPLNMMLPCMMLPMCRMTPPSACMSAMCHawkesPoisson.json.png}
     \end{subfigure}
    \hfill
    \begin{subfigure}[b]{0.32\textwidth}
         \centering
         \includegraphics[width=\textwidth]{images/cd_diag/stat_tests_holm_F1-score_marked_CPLNMMLPCMMLPMCRMTPPSACMSAMCHawkesPoisson.json.png}
     \end{subfigure}
     \vfill\vspace{-0.6cm}
     \begin{subfigure}[b]{0.32\textwidth}
         \centering
         \includegraphics[width=\textwidth]{images/cd_diag/stat_tests_holm_NLLMark_marked_+ BNo B.json.png}
     \end{subfigure}
     \hfill
     \begin{subfigure}[b]{0.32\textwidth}
         \centering
         \includegraphics[width=\textwidth]{images/cd_diag/stat_tests_holm_MarkCal._marked_+ BNo B.json.png}
     \end{subfigure}
    \hfill
    \begin{subfigure}[b]{0.32\textwidth}
         \centering
         \includegraphics[width=\textwidth]{images/cd_diag/stat_tests_holm_F1-score_marked_+ BNo B.json.png}
     \end{subfigure}

     \vspace{-0.8cm}
\label{fig:class_reddit_lasftm}
\caption{Critical Distance (CD) diagrams per component on the Mark NLL (left-hand column), ECE (middle column) and F1-score (right column) for marked datasets. A bold line joins models variations that are not statistically different.}
\label{Distribution}
\end{figure}
\end{center}
